# Supplementary material for: AI-aided Geometric Design of Anti-infection Catheters
Source: arXiv:2304.14554 source file (2023-04-27)
Supplement: Supplementary file 1 [file S1-supplements.tex]

% \bmhead{Supplementary information}

% If your article has accompanying supplementary file/s please state so here. 

% Authors reporting data from electrophoretic gels and blots should supply the full unprocessed scans for key as part of their Supplementary information. This may be requested by the editorial team/s if it is missing.

% Please refer to Journal-level guidance for any specific requirements.
